# Supplementary material for: OmniSat: Self-Supervised Modality Fusion for Earth Observation
Source: arXiv:2404.08351 source file (2024-07-17)
Supplement: Supplementary file 1 [file suppmat.tex]

\input{figures/visualizer}

In this document, we introduce our interactive visualization tool (\secref{sec:visu}), XXXX

%==============================================
\section{Interactive Visualization}
%==============================================
\label{sec:visu}

We release for this project an interactive visualization tool 
{which produces} HTML files compatible with any browser. As shown in 
{\figref{fig:visu},}
we can visualize samples from the datasets with different point attributes and from any angle. These visualizations were instrumental in designing and validating our model, and we hope that they will be help the reader's understanding as well.

%==============================================
\section{Source Code}
%==============================================
\label{sec:code}

% We make our source code available to the reader, along with indications for installing the project and reproducing our main results on S3DIS, KITTI-360, and DALES. 
% This code will be publicly released upon publication.
{
We make our source code publicly available at \GITHUB.
The code provides all necessary instructions for installing and navigating the project, simple commands to reproduce our main results on all datasets, off-the-shelf pretrained models, and ready-to-use notebooks. 
}
Our method is developed in Pytorch and relies on the libraries PyTorch Geometric, PyTorch Lightning, and Hydra. 

%==============================================
\section{Limitations}
%==============================================
\label{sec:limitations}

%==============================================
\section{Implementation Details}
%==============================================
\label{sec:implem}

\subsection{UT&T \cite{garioud2023flair}}

% Pour moi ces info ci dessous vont aller dans le sup mat 
The UNet of UT\&T has a ResNet-34 backbone partially initialized with a RGB ResNet pre-trained on ImageNet but it is not the case for the UTAE branches. 

%In the case of PASTIS-HD, the cloudy images can not be filtered out because this information is not available. 
In the case of TreeSat AI, the aerial image are resized to (as the UNet need a input size multiple of 32). The UTAE branches are reduced to a smaller size due to the small size of the Sentinel images. 
All the model are trained for 100 epochs monitored by an early stoppping with a patience of 30 epochs on the validation loss (of all the modalities). 

%We also average the S1 time series per month on both Pastis-HD and TreeSatAI-TS.

%For Pastis-HD, we Split the image into 8 sub images for PASTIS-R due to memory issues.

%==============================================
\section{Detailed Results}
%==============================================
\label{sec:classwise}

\input{tables/classwise}

We report in \tabref{tab:classwise} the class-wise performance across all datasets for \SHORTHAND and other methods for which this information was available. 

\balance

\input{tables/colormaps}

%==============================================
%==============================================
%\section{Supplementary Visualization}
%==============================================
%extra vizs: failure cases
%only if you have time
